# Supplementary material for: SciDataCopilot: An Agentic Data Preparation Framework for AGI-driven Scientific Discovery
Source: arXiv:2602.09132 source file (2026-02-09)
Supplement: Supplementary file 1 [file X-appendix.tex]

\newpage
% \appendix

\section*{Authors}
\addcontentsline{toc}{section}{Authors}
% \subsection{Authors}

\textbf{Co-first Authors}

Jiyong Rao, Yicheng Qiu, Jiahui Zhang, Juntao Deng, Shangquan Sun

\textbf{Contributors}

% ai4neuro
% 伍佳敏，郑启豪，刘棉莘，朱宇
Jiamin Wu, Qihao Zheng, Mianxin Liu, Yu Zhu,
% ai4s
% 零丰华、张铂、张文龙、唐诗翔、董楠卿、李玉强、王潚崧、周东展
Fenghua Ling, Hao Chen, Bo Zhang, Wenlong Zhang, Shixiang Tang, Nanqing Dong, Yuqiang Li, Xiaosong Wang, Dongzhan Zhou,
% others
% 何聪辉、王广宇、吴郦军，邵婧、汪旭鸿
Conghui He, Guangyu Wang, Lijun Wu, Jing Shao, Xuhong Wang,
Wanli Ouyang

\textbf{Corresponding Authors}

Runkai Zhao, Chunfeng Song, Lei Bai, Chi Zhang

\textbf{Project Leader}

Chi Zhang

\textbf{Main Affiliations}

Shanghai Artificial Intelligence Laboratory
